# Supplementary material for: Thickness-dependent electron momentum relaxation times in thin iron films
Source: arXiv:1905.06739 ancillary file (2019-05-16)
Supplement: Supplementary file 1 [file SupplementaryMaterialThicknessDependentRelaxationTimes.pdf]

Supplementary information for “Thickness-dependent electron momentum relaxation times in thin iron films”.

## S1: Sample preparation

The iron films were deposited on double polished MgO (100) substrates and capped with ca. 12 nm of MgO. The molecular beam epitaxy was performed at room temperature with subsequent annealing at 600 K. The deposition rate was 0.05 nm/min at standard $10^{-10}$ Torr ($10^{-8}$ Pa) pressure. The thicknesses were controlled “in situ” by quartz balance sensing and confirmed by small-angle x-ray diffraction (XRD) for selected samples by means of a Rigaku SmartLab X-ray diffractometer equipped with a monochromatic source (Ge(220)×2) delivering a Cu Kα1 incident beam (45 kV, 200 mA, λ = 0.154056 nm), see Figure SM1). Roughnesses extracted from XRD average 0.9 ± 0.1 nm, without significant dependence on thickness. Reflection high energy electron

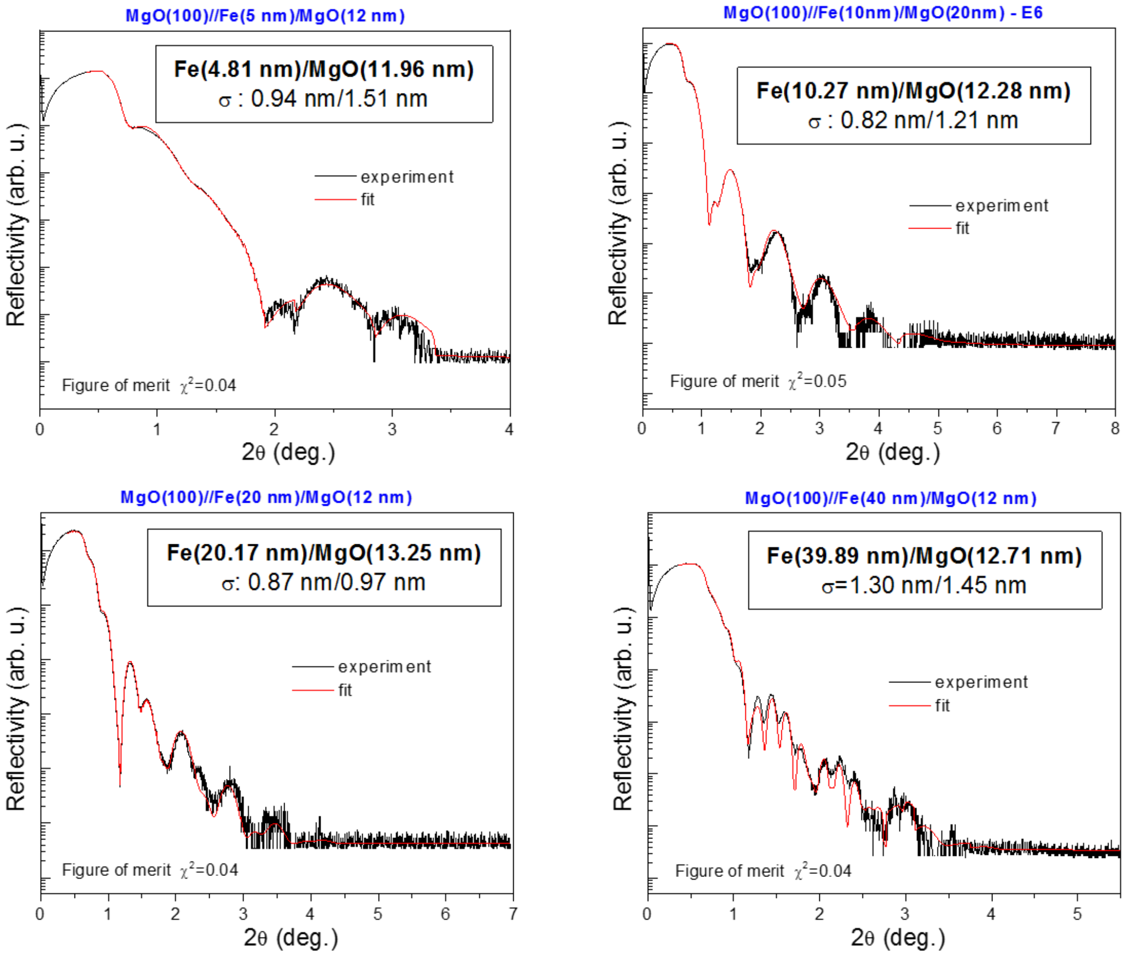


**Figure SM1**. X-Ray reflectivity measurement of selected Fe thin films. The recovered thicknesses are given in parenthesis behind the layer materials. Below them, the respective roughnesses $\sigma$ are displayed. Experimental data points are shown in black, while the fit in red with a maximum figure of merit $\chi 2$ = 0.05.

diffraction images indicate that this preparation method achieves single-crystalline films with bcc lattice structure (see Figure SM2 and SM3).

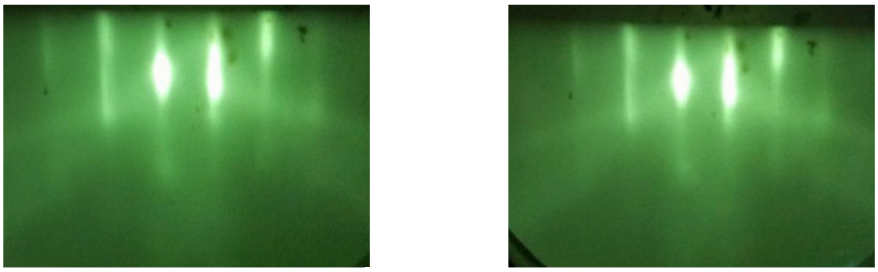

**Figure SM2:** RHEED images of Fe on MgO/MgO epitaxial uptake /Fe

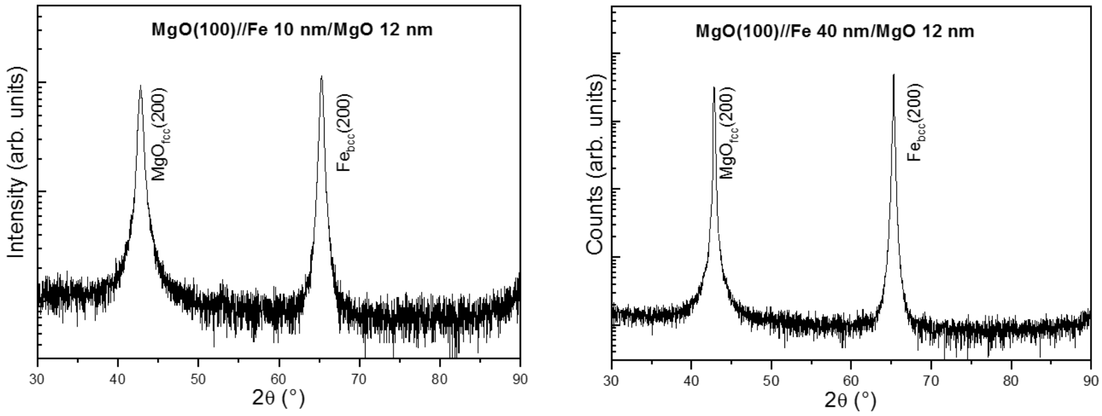


**Figure SM3.** X-Ray diffraction pattern of selected Fe thin layers, Fe crystallizes well in the bcc structure.

## S2: Extraction of THz conductivity spectra from field transmission spectra

We note that this is the first time, to the best of our knowledge, that the complex conductivity has been recovered for "non-thin" metal films, that is films which the complex phase acquired by the terahertz field during a direct transit is non-negligible. We have expanded the substrate thickness correction determination we presented in a previous work[1] accordingly, but this yields deviations smaller than the statistical error. However, the full transfer matrix approach for recovering the

complex conductivity is crucial for all films thicker than 20 nm, because the thicker the film, the smaller the conductivity phase and therefore the current response time would appear in the conventionally used thin film approximation.

## S3: Extraction of decay time and DC-conductivity from THz conductivity spectra

We extract the current response times and DC conductivities of the effective Drude model (eq. 3). The frequency range between 0.6 and 2.0 THz has the best phase resolution. We solve the complex conductivity at each frequency for response time and DC-conductivity in this region. The resulting values are similar for all frequencies, but the values vary more than their standard errors from repeated measurements predict. We note that the discrepancies correlate between samples referenced to the same substrate. We suspect contamination/roughness of the reference substrates as main cause for these small discrepancies. We extract the current response times and DC-conductivities by averaging over the entire frequency range. Experimental noise, discrepancies between frequencies and discrepancies between measurements a year apart at slightly different positions have been factored into the parameters and error estimates.


1. Krewer, K. L. *et al.* Accurate terahertz spectroscopy of supported thin films by precise substrate thickness correction. *Opt. Lett.* **43**, 447–450 (2018).
